# Supplementary material for: Ocean dynamics of outer solar system satellites
Source: arXiv:1901.04093 source file (2019-07-22)
Supplement: Supplementary file 1 [file Soderlund_GRL_Supporting-Information_v3.pdf]

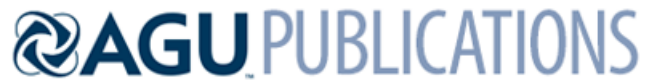

*Geophysical Research Letters*

Supporting Information for

**Ocean dynamics of outer solar system satellites**

K. M. Soderlund

Institute for Geophysics, Jackson School of Geosciences, The University of Texas at Austin, Austin, Texas, USA

**Contents of this file**

Figures S1 to S3

**Introduction**

Below are three figures showing (1) the convective regime diagram from Figure 1 zoomed in on each satellite and the numerical models and (2) modeling results from the suite of numerical models that vary the Rayleigh number for fixed Ekman and Prandtl numbers.

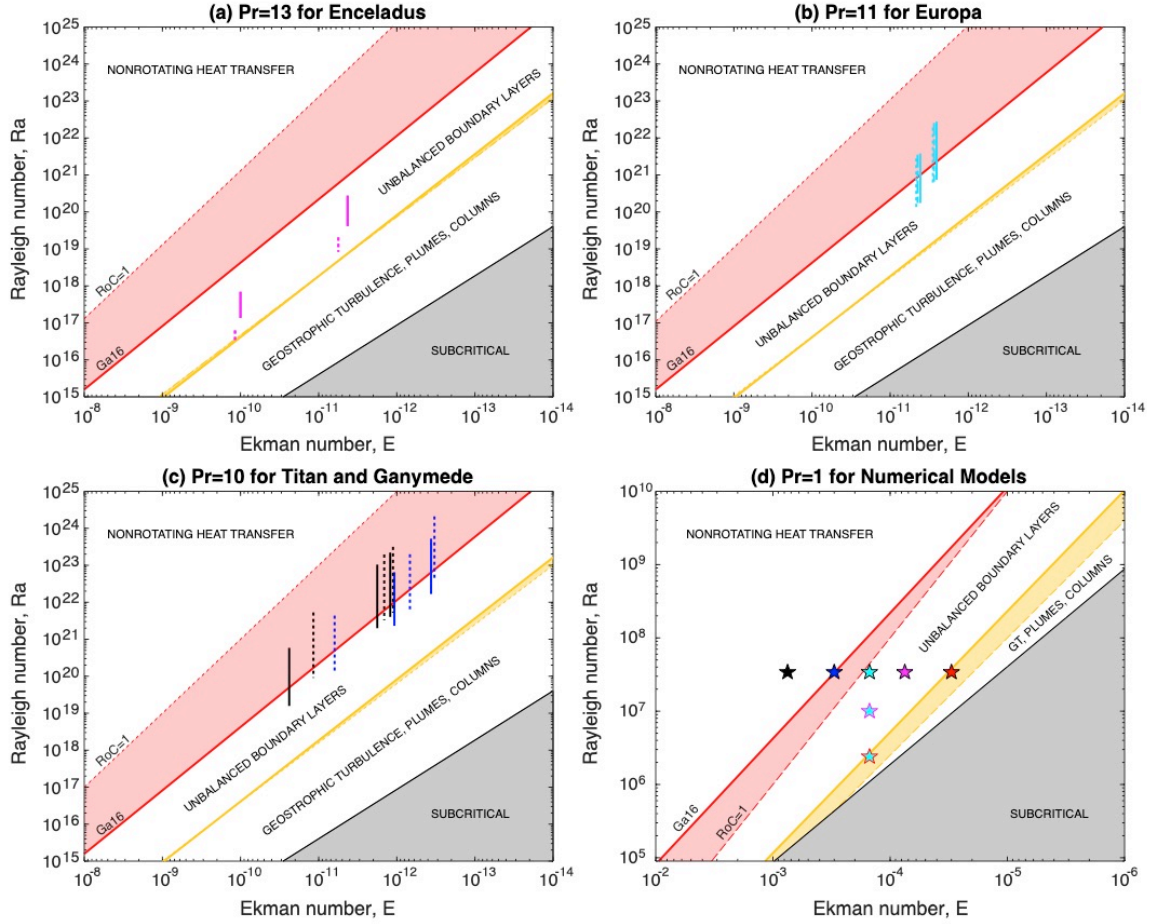

**Figure S1.** Convective regime diagram following Cheng et al. (2018) zoomed in on (a) Enceladus, (b) Europa, (c) Titan and Ganymede, and (d) the numerical models. In (a), magenta vertical lines denote the  $Ra$ - $E$  estimates for Enceladus assuming thick and thin outer ice shells; solid lines denote an  $MgSO_4$  (10 wt %) composition and dashed lines denote seawater. Pure water was also considered but has  $\alpha < 0$  and is therefore stable to convection. In (b), cyan vertical lines denote the  $Ra$ - $E$  estimates for Europa assuming thick and thin outer ice shells; solid lines denote an  $MgSO_4$  (10 wt %) composition, dashed lines denote seawater, and dotted lines denote pure water. In (c), black (blue) vertical lines denote the  $Ra$ - $E$  estimates for Titan (Ganymede) assuming thick, intermediate, and thin outer ice shells; solid lines denote an  $MgSO_4$  (10 wt %) composition and dotted lines denote pure water. In (d), numerical simulations are denoted by stars, where interior color denotes Ekman number and exterior color denotes Rayleigh number. Interior: red ( $E = 3.0 \times 10^{-5}$ ), magenta ( $E = 7.5 \times 10^{-5}$ ), cyan ( $E = 1.5 \times 10^{-4}$ ), blue ( $E = 3.0 \times 10^{-4}$ ), and black ( $E = 7.5 \times 10^{-4}$ ). Exterior: black ( $Ra = 3.4 \times 10^7$ ), magenta ( $Ra = 1.0 \times 10^7$ ), and red ( $Ra = 2.4 \times 10^6$ ). In all panels, the black diagonal line denotes the scaling for the onset of convection (Chandrasekhar, 1961), the yellow lines bound the range of predicted transitions from the GT regime to the UBL regime (Ecke & Niemela, 2014; Julien et al., 2012), and the red lines bound the range of predicted transitions from the UBL regime to the NR regime (Gastine et al., 2016; Gilman, 1977) using the same line conventions as Figure 1.

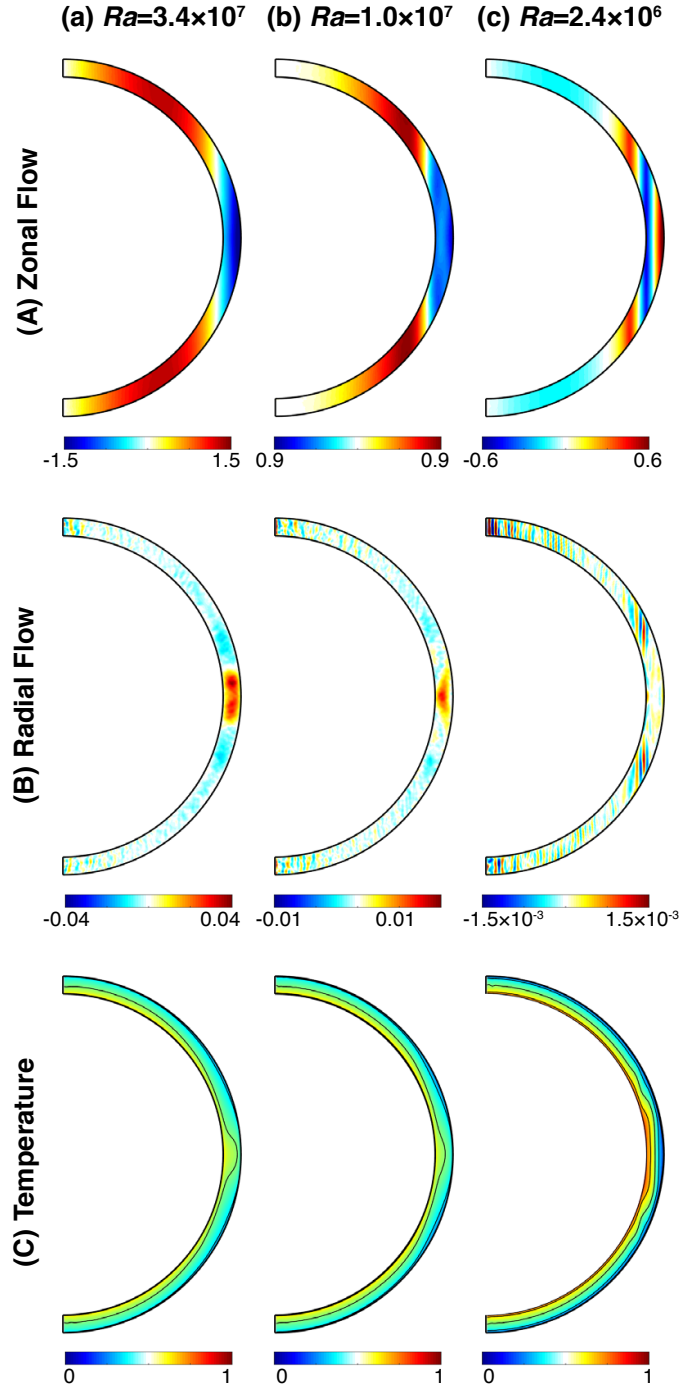

**Figure S2.** Mean velocity and temperature fields averaged over all longitudes and at least 0.02 viscous diffusion times for each model in the Rayleigh number suite. (A) Zonal flows given in dimensionless Rossby number units,  $Ro=U/\Omega D$ , which characterizes the ratio of rotational to inertial timescales. Red (blue) denotes prograde (retrograde) currents. (B) Radial flows given in  $Ro$  units. Red (blue) denotes upwelling (downwelling) currents. (C) Superadiabatic temperature in dimensionless units with isotherm contours superimposed (interval of 0.2). Red (blue) denotes warm (cool) fluid.

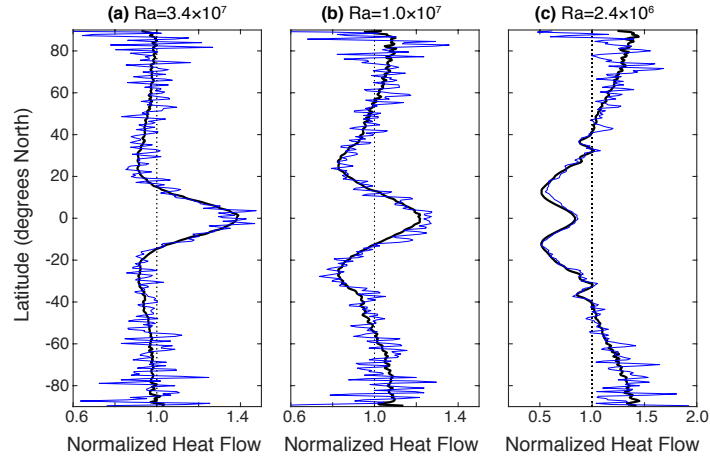

**Figure S3.** Heat flux along the outer boundary normalized by the mean value for each model in the Rayleigh number suite. Black lines denote the average over all longitudes and at least 0.02 viscous diffusion times; blue lines show azimuthal averages at snapshots in time.
